# Supplementary material for: Can LLMs plan paths with extra hints from solvers?
Source: arXiv:2410.05045 source file (2024-10-07)
Supplement: Supplementary file 1 [file appendices.tex]

\section{Appendix}
\subsection{Prompting details}
\label{sec:prompt_details}

The initial prompt for explaining the path planning problem is as follows:

\begin{verbatim}
    We are going to solve ... 
\end{verbatim}

\subsection{Other tables}
\subsubsection{}
\begin{table*}[h!]
\centering
\begin{tabular}{ccc}
\toprule
\textbf{Environment} & \textbf{Result} & \textbf{Success Rate}  \\ \midrule
\multicolumn{3}{c}{\textbf{Solvable Versions}} \\ \midrule
\textbf{Box}          & 10 Correct & 100\% \\
\textbf{Box Boundary} & 10 Correct & 100\% \\
\textbf{Canyon}       & 9 Correct &  90\% \\
\textbf{Curve}        & 8 Correct &  80\% \\
\textbf{Diagonal Wall}& 10 Correct & 100\% \\
\textbf{Easy}         & 10 Correct & 100\% \\
\textbf{Maze 2D}      & 8 Correct &  80\% \\
\textbf{Scots HSCC16} & 8 Correct &  80\% \\
\textbf{Spiral}       & 9 Correct &  90\% \\
\textbf{Wall}         & 10 Correct & 100\% \\ \midrule
\multicolumn{3}{c}{\textbf{Unsolvable Versions}} \\ \midrule
\textbf{Box}          & 10 Incorrect & 0\% \\
\textbf{Box II}       & 10 Incorrect & 0\% \\
\textbf{Canyon}       & 10 Incorrect & 0\% \\
\textbf{Curve}        & 1 Correct, 9 Incorrect & 10\% \\
\textbf{Diagonal Wall}& 10 Incorrect & 0\% \\
\textbf{Easy}         & 10 Incorrect & 0\% \\
\textbf{Maze 2D}      & 10 Incorrect & 0\% \\
\textbf{Scots HSCC16} & 1 Correct, 9 Incorrect & 10\% \\
\textbf{Spiral}       & 1 Correct, 9 Incorrect & 10\% \\
\textbf{Wall}         & 10 Incorrect & 0\% \\ \midrule
\textbf{Average}      & \multicolumn{2}{c}{Solvable: 92.00\% Correct} \\
\textbf{Average}      & \multicolumn{2}{c}{Unsolvable: 3.00\% Correct} \\
\bottomrule
\end{tabular}
\caption{Experiment: Identify solvable or not. Model: llama-3.1-70b-versatile. Prompting strategy: solvable\_prompt.}
\label{table:results2}
\end{table*}

\begin{figure*}
    \centering

\begin{table}[H]
\centering
\begin{tabular}{lccccccccc}
\toprule
\textbf{Problem} & \multicolumn{3}{c}{\textbf{Gemini Pro 1.5}} & \multicolumn{3}{c}{\textbf{GPT-4o}} & \multicolumn{3}{c}{\textbf{Claude Sonnet 3.5}} \\ 
\cmidrule(lr){2-4} \cmidrule(lr){5-7} \cmidrule(lr){8-10}              
                    & \textbf{S\%} & \textbf{N} & \textbf{PL} 
                    & \textbf{S\%} & \textbf{N} & \textbf{PL Succ.} 
                    & \textbf{S\%} & \textbf{N} & \textbf{PL} \\ 
\midrule
\textbf{Box}             & 90  & 8.80  & 6.33  & 50\%  & 17.30 & 8.00  & 30  & 17.33 & 5.00  \\ 
\textbf{Box B.}    & 100 & 1.30  & 3.70  & 100\% & 1.00  & 3.90  & 100 & 1.20  & 4.10  \\ 
\textbf{Canyon}          & 30  & 15.90 & 5.33  & 100\% & 2.60  & 4.60  & 80  & 5.62  & 5.88  \\ 
\textbf{Curve}           & 30  & 17.90 & 11.00 & 100\% & 4.30  & 5.80  & 20  & 16.50 & 8.50  \\ 
\textbf{D. Wall}   & 90  & 8.90  & 7.78  & 0\%   & 20.00 & -     & 0   & -     & -     \\ 
\textbf{Easy}            & 100 & 3.90  & 6.60  & 100\% & 6.40  & 5.60  & 20  & 12.50 & 6.00  \\ 
\textbf{Maze}            & 10  & 20.10 & 13.00 & 0\%   & 20.00 & -     & 0   & -     & -     \\ 
\textbf{Scots}           & 0   & -     & -     & 10\%  & 18.70 & 10.00 & 0   & -     & -     \\ 
\textbf{Spiral}          & 30  & 17.10 & 9.00  & 0\%   & 20.00 & -     & 0   & -     & -     \\ 
\textbf{Wall}            & 100 & 8.00  & 6.50  & 100\% & 5.40  & 6.90  & 10  & 20.00 & 7.00  \\ 
\midrule
\textbf{1 Obs}      & 100 & 1.90  & 4.80  & 70\%  & 1.86  & 5.14  & 55  & 2.18  & 4.45  \\ 
\textbf{2 Obs}     & 60  & 2.83  & 6.33  & 50\%  & 2.60  & 5.50  & 35  & 1.43  & 4.14  \\ 
\textbf{3 Obs}     & 65  & 4.15  & 6.77  & 20\%  & 2.25  & 6.25  & 20  & 3.25  & 5.75  \\ 
\textbf{4 Obs}     & 20  & 5.00  & 7.50  & 10\%  & 5.50  & 9.00  & 10  & 2.00  & 4.00  \\ 
\textbf{5 Obs}     & 35  & 3.86  & 6.86  & 15\%  & 3.00  & 7.00  & 15  & 5.33  & 6.00  \\ 
\bottomrule
\end{tabular}
\caption{Comparison of performance metrics across different environments for Gemini Pro 1.5, GPT-4o, and Claude Sonnet 3.5.}
\label{table:merged_results}
\end{table}

\begin{table}[H]
\centering
\begin{tabular}{lccccccccc}
\toprule
 & \multicolumn{3}{c}{\textbf{Gemini Pro 1.5}} & \multicolumn{3}{c}{\textbf{GPT-4o}} & \multicolumn{3}{c}{\textbf{Claude Sonnet 3.5}} \\ 
\cmidrule(lr){2-4} \cmidrule(lr){5-7} \cmidrule(lr){8-10}              
                    \textbf{Problem} & \textbf{Success R.} & \textbf{Iter. Succ.} & \textbf{PL Succ.} 
                    & \textbf{Success R.} & \textbf{Iter. Succ.} & \textbf{PL Succ.} 
                    & \textbf{Success R.} & \textbf{Iter. Succ.} & \textbf{PL Succ.} \\ 
\midrule
\textbf{Easy}            & 100\% & 3.90  & 6.60  & 100\% & 6.40  & 5.60  & 20\%  & 12.50 & 6.00  \\ 
\textbf{Box B.}    & 100\% & 1.30  & 3.70  & 100\% & 1.00  & 3.90  & 100\% & 1.20  & 4.10  \\ 
\textbf{Wall}            & 100\% & 8.00  & 6.50  & 100\% & 5.40  & 6.90  & 10\%  & 20.00 & 7.00  \\ 
\textbf{Box}             & 90\%  & 8.80  & 6.33  & 50\%  & 17.30 & 8.00  & 30\%  & 17.33 & 5.00  \\ 
\textbf{Canyon}          & 30\%  & 15.90 & 5.33  & 100\% & 2.60  & 4.60  & 80\%  & 5.62  & 5.88  \\ 
\textbf{D. Wall}   & 90\%  & 8.90  & 7.78  & 0\%   & 20.00 & -     & 0\%   & -     & -     \\ 
\textbf{Curve}           & 30\%  & 17.90 & 11.00 & 100\% & 4.30  & 5.80  & 20\%  & 16.50 & 8.50  \\ 
\textbf{Spiral}          & 30\%  & 17.10 & 9.00  & 0\%   & 20.00 & -     & 0\%   & -     & -     \\ 
\textbf{Maze}            & 10\%  & 20.10 & 13.00 & 0\%   & 20.00 & -     & 0\%   & -     & -     \\ 
\textbf{Scots}           & 0\%   & -     & -     & 10\%  & 18.70 & 10.00 & 0\%   & -     & -     \\ 
\midrule
\textbf{1 Obs}      & 100\% & 1.90  & 4.80  & 70\%  & 1.86  & 5.14  & 55\%  & 2.18  & 4.45  \\ 
\textbf{2 Obs}     & 60\%  & 2.83  & 6.33  & 50\%  & 2.60  & 5.50  & 35\%  & 1.43  & 4.14  \\ 
\textbf{3 Obs}     & 65\%  & 4.15  & 6.77  & 20\%  & 2.25  & 6.25  & 20\%  & 3.25  & 5.75  \\ 
\textbf{4 Obs}     & 20\%  & 5.00  & 7.50  & 10\%  & 5.50  & 9.00  & 10\%  & 2.00  & 4.00  \\ 
\textbf{5 Obs}     & 35\%  & 3.86  & 6.86  & 15\%  & 3.00  & 7.00  & 15\%  & 5.33  & 6.00  \\ 
\bottomrule
\end{tabular}
\end{table}

\begin{table}[H]
\centering
\begin{tabular}{lccccccccc}
\toprule
& \multicolumn{3}{c}{\textbf{Gemini}} & \multicolumn{3}{c}{\textbf{GPT-4o}} & \multicolumn{3}{c}{\textbf{Claude}} \\ 
\cmidrule(lr){2-4} \cmidrule(lr){5-7} \cmidrule(lr){8-10}              
\textbf{Problem} & \textbf{SR\%} & \textbf{IS} & \textbf{PL} 
                    & \textbf{SR\%} & \textbf{IS} & \textbf{PL} 
                    & \textbf{SR\%} & \textbf{IS} & \textbf{PL} \\ 
\midrule
\textbf{Easy}            & 100 & 3.9  & 6.6  & 100 & 6.4  & 5.6  & 20 & 12.5 & 6.0  \\ 
\textbf{Box B.}    & 100 & 1.3  & 3.7  & 100 & 1.0  & 3.9  & 100 & 1.2  & 4.1  \\ 
\textbf{Wall}            & 100 & 8.0  & 6.5  & 100 & 5.4  & 6.9  & 10 & 20.0 & 7.0  \\ 
\textbf{Box}             & 90 & 8.8  & 6.3  & 50  & 17.3 & 8.0  & 30 & 17.3 & 5.0  \\ 
\textbf{Canyon}          & 30  & 15.9 & 5.3  & 100 & 2.6  & 4.6  & 80 & 5.6  & 5.9  \\ 
\textbf{D. Wall}   & 90  & 8.9  & 7.8  & 0   & 20.0 & -     & 0  & -     & -     \\ 
\textbf{Curve}           & 30  & 17.9 & 11.0 & 100 & 4.3  & 5.8  & 20 & 16.5 & 8.5  \\ 
\textbf{Spiral}          & 30  & 17.1 & 9.0  & 0   & 20.0 & -     & 0  & -     & -     \\ 
\textbf{Maze}            & 10  & 20.1 & 13.0 & 0   & 20.0 & -     & 0  & -     & -     \\ 
\textbf{Scots}           & 0   & -     & -     & 10  & 18.7 & 10.0 & 0  & -     & -     \\ 
\midrule
\textbf{1 Obs}      & 100 & 1.9  & 4.8  & 70  & 1.9  & 5.1  & 55 & 2.2  & 4.5  \\ 
\textbf{2 Obs}     & 60  & 2.8  & 6.3  & 50  & 2.6  & 5.5  & 35 & 1.4  & 4.1  \\ 
\textbf{3 Obs}     & 65  & 4.2  & 6.8  & 20  & 2.3  & 6.3  & 20 & 3.3  & 5.8  \\ 
\textbf{4 Obs}     & 20  & 5.0  & 7.5  & 10  & 5.5  & 9.0  & 10 & 2.0  & 4.0  \\ 
\textbf{5 Obs}     & 35  & 3.9  & 6.9  & 15  & 3.0  & 7.0  & 15 & 5.3  & 6.0  \\ 
\bottomrule
\end{tabular}
\end{table}

\end{figure*}

\begin{itemize}

    \item \textcolor{red}{Gemini 1.5 pro}
    \begin{table}[H]
    \centering
    \begin{tabular}{lcccccc}
    \toprule
    \textbf{Environment}     & \textbf{Success R.} & \textbf{Iter. Succ.} & \textbf{Path Len.} & \textbf{PL Succ.} \\ 
    \midrule
    \textbf{Box}             & 90\%             & 10.89               & 4.50               & 4.44              \\ 
    \textbf{Box Boundary}    & 100\%            & 1.30                & 3.70               & 3.70              \\ 
    \textbf{Canyon}          & 0\%              & -                   & 4.90               & -                 \\ 
    \textbf{Curve}           & 40\%             & 8.00                & 5.50               & 6.50              \\ 
    \textbf{Diagonal Wall}   & 70\%             & 8.86                & 4.90               & 5.00              \\ 
    \textbf{Easy}            & 100\%            & 3.30                & 4.50               & 4.50              \\ 
    \textbf{Maze 2D}         & 0\%              & -                   & 6.80               & -                 \\ 
    \textbf{Scots HSCC16}    & 20\%             & 13.50               & 14.40              & 12.50             \\ 
    \textbf{Spiral}          & 60\%             & 14.17               & 6.10               & 6.17              \\ 
    \textbf{Wall}            & 100\%            & 1.60                & 4.20               & 4.20              \\ 
    \midrule
    \textbf{1 Obstacle} & 95\% & 1.74 & 4.25 & 4.11 \\
    \textbf{2 Obstacles} & 95\% & 2.53 & 4.90 & 4.89 \\
    \textbf{3 Obstacles} & 75\% & 2.87 & 5.30 & 4.87 \\
    \textbf{4 Obstacles} & 45\% & 3.67 & 5.45 & 4.89 \\
    \textbf{5 Obstacles} & 30\% & 3.67 & 5.70 & 4.83 \\
        
    \bottomrule
    \end{tabular}
    \caption{Man runtime: 03h:33m:23s, Random runtime:  01h:01m:23s}
    \label{table:results_summary1}
    \end{table}

    \item GPT-4o (add random table (gpt\_full\_path)
    \begin{table}[H]
    \centering
    \begin{tabular}{lcccccc}
    \toprule
    \textbf{Environment} & \textbf{Success R.} & \textbf{Iter. Succ.} & \textbf{Path Len.} & \textbf{PL Succ.} \\ 
    \midrule
    \textbf{Box}             & 50\%             & 8.60               & 4.90               & 5.20              \\ 
    \textbf{Box Boundary}    & 100\%            & 1.00               & 3.00               & 3.00              \\ 
    \textbf{Canyon}          & 100\%            & 2.20               & 4.70               & 4.70              \\ 
    \textbf{Curve}           & 70\%             & 9.14               & 5.60               & 5.43              \\ 
    \textbf{Diagonal Wall}   & 0\%              & -              & 4.60               & -1.00             \\ 
    \textbf{Easy}            & 100\%            & 2.60               & 5.20               & 5.20              \\ 
    \textbf{Maze 2D}         & 0\%              & -              & 6.60               & -1.00             \\ 
    \textbf{Scots HSCC16}    & 0\%              & -              & 9.10               & -1.00             \\ 
    \textbf{Spiral}          & 0\%              & -              & 5.30               & -1.00             \\ 
    \textbf{Wall}            & 100\%            & 1.60               & 4.50               & 4.50              \\ 
    \midrule
    \textbf{1 Obstacle} & 90.00\% & 1.67 & 5.15 & 4.94 \\
    \textbf{2 Obstacles} & 50.00\% & 2.30 & 6.95 & 5.70 \\
    \textbf{3 Obstacles} & 15.00\% & 4.00 & 7.10 & 6.33 \\
    \textbf{4 Obstacles} & 5.00\%  & 1.00 & 8.00 & 5.00 \\
    \textbf{5 Obstacles} & 10.00\% & 3.00 & 7.80 & 7.00 \\
    \bottomrule
    \end{tabular}
    \caption{Max iterations: 20, Runtime: 02h:50m:27s; Number of iterations: 5, Evaluations per Env: 20, Runtime: 01h:13m:09s}
    \label{table:results_summary2}
    \end{table}

\item{Claude 3.5}
\begin{table}[H]
\centering
\begin{tabular}{lcccccc}
\toprule
\textbf{Environment} & \textbf{Success R.} & \textbf{Iter. Succ.} & \textbf{Path Len.} & \textbf{PL Succ.} \\ 
\midrule
\textbf{Box}             & 0\%              & -              & 4.60               & -1.00             \\ 
\textbf{Box Boundary}    & 100\%            & 1.00               & 3.60               & 3.60              \\ 
\textbf{Canyon}          & 70\%             & 7.14               & 5.90               & 5.71              \\ 
\textbf{Curve}           & 10\%             & 3.00               & 12.60              & 9.00              \\ 
\textbf{Diagonal Wall}   & 0\%              & -              & 4.60               & -1.00             \\ 
\textbf{Easy}            & 0\%              & -              & 4.40               & -1.00             \\ 
\textbf{Maze 2D}         & 0\%              & -              & 16.40              & -1.00             \\ 
\textbf{Scots HSCC16}    & 0\%              & -              & 11.60              & -1.00             \\ 
\textbf{Spiral}          & 0\%              & -              & 4.50               & -1.00             \\ 
\textbf{Wall}            & 10\%             & 11.00              & 5.10               & 5.00              \\ 
\midrule
\textbf{1 Obstacle} & 85.00\% & 1.94 & 4.65 & 4.53 \\
\textbf{2 Obstacles} & 60.00\% & 1.75 & 5.05 & 4.33 \\
\textbf{3 Obstacles} & 25.00\% & 3.40 & 5.50 & 4.60 \\
\textbf{4 Obstacles} & 0.00\%  & -1.00 & 6.15 & -1.00 \\
\textbf{5 Obstacles} & 15.00\% & 3.00 & 6.45 & 5.00 \\
\bottomrule
\end{tabular}
\caption{Max iterations: 20, Runtime comparison of random environments and manual settings.}
\end{table}

\end{itemize}
